# Supplementary material for: Diversified Multiscale Graph Learning with Graph Self-Correction
Source: arXiv:2103.09754 source file (2021-03-17)
Supplement: Supplementary file 1 [file appendix-demo.tex]

\begin{figure*} [h]
  \centering
  % Requires \usepackage{graphicx}
  \includegraphics[width=0.7\linewidth]{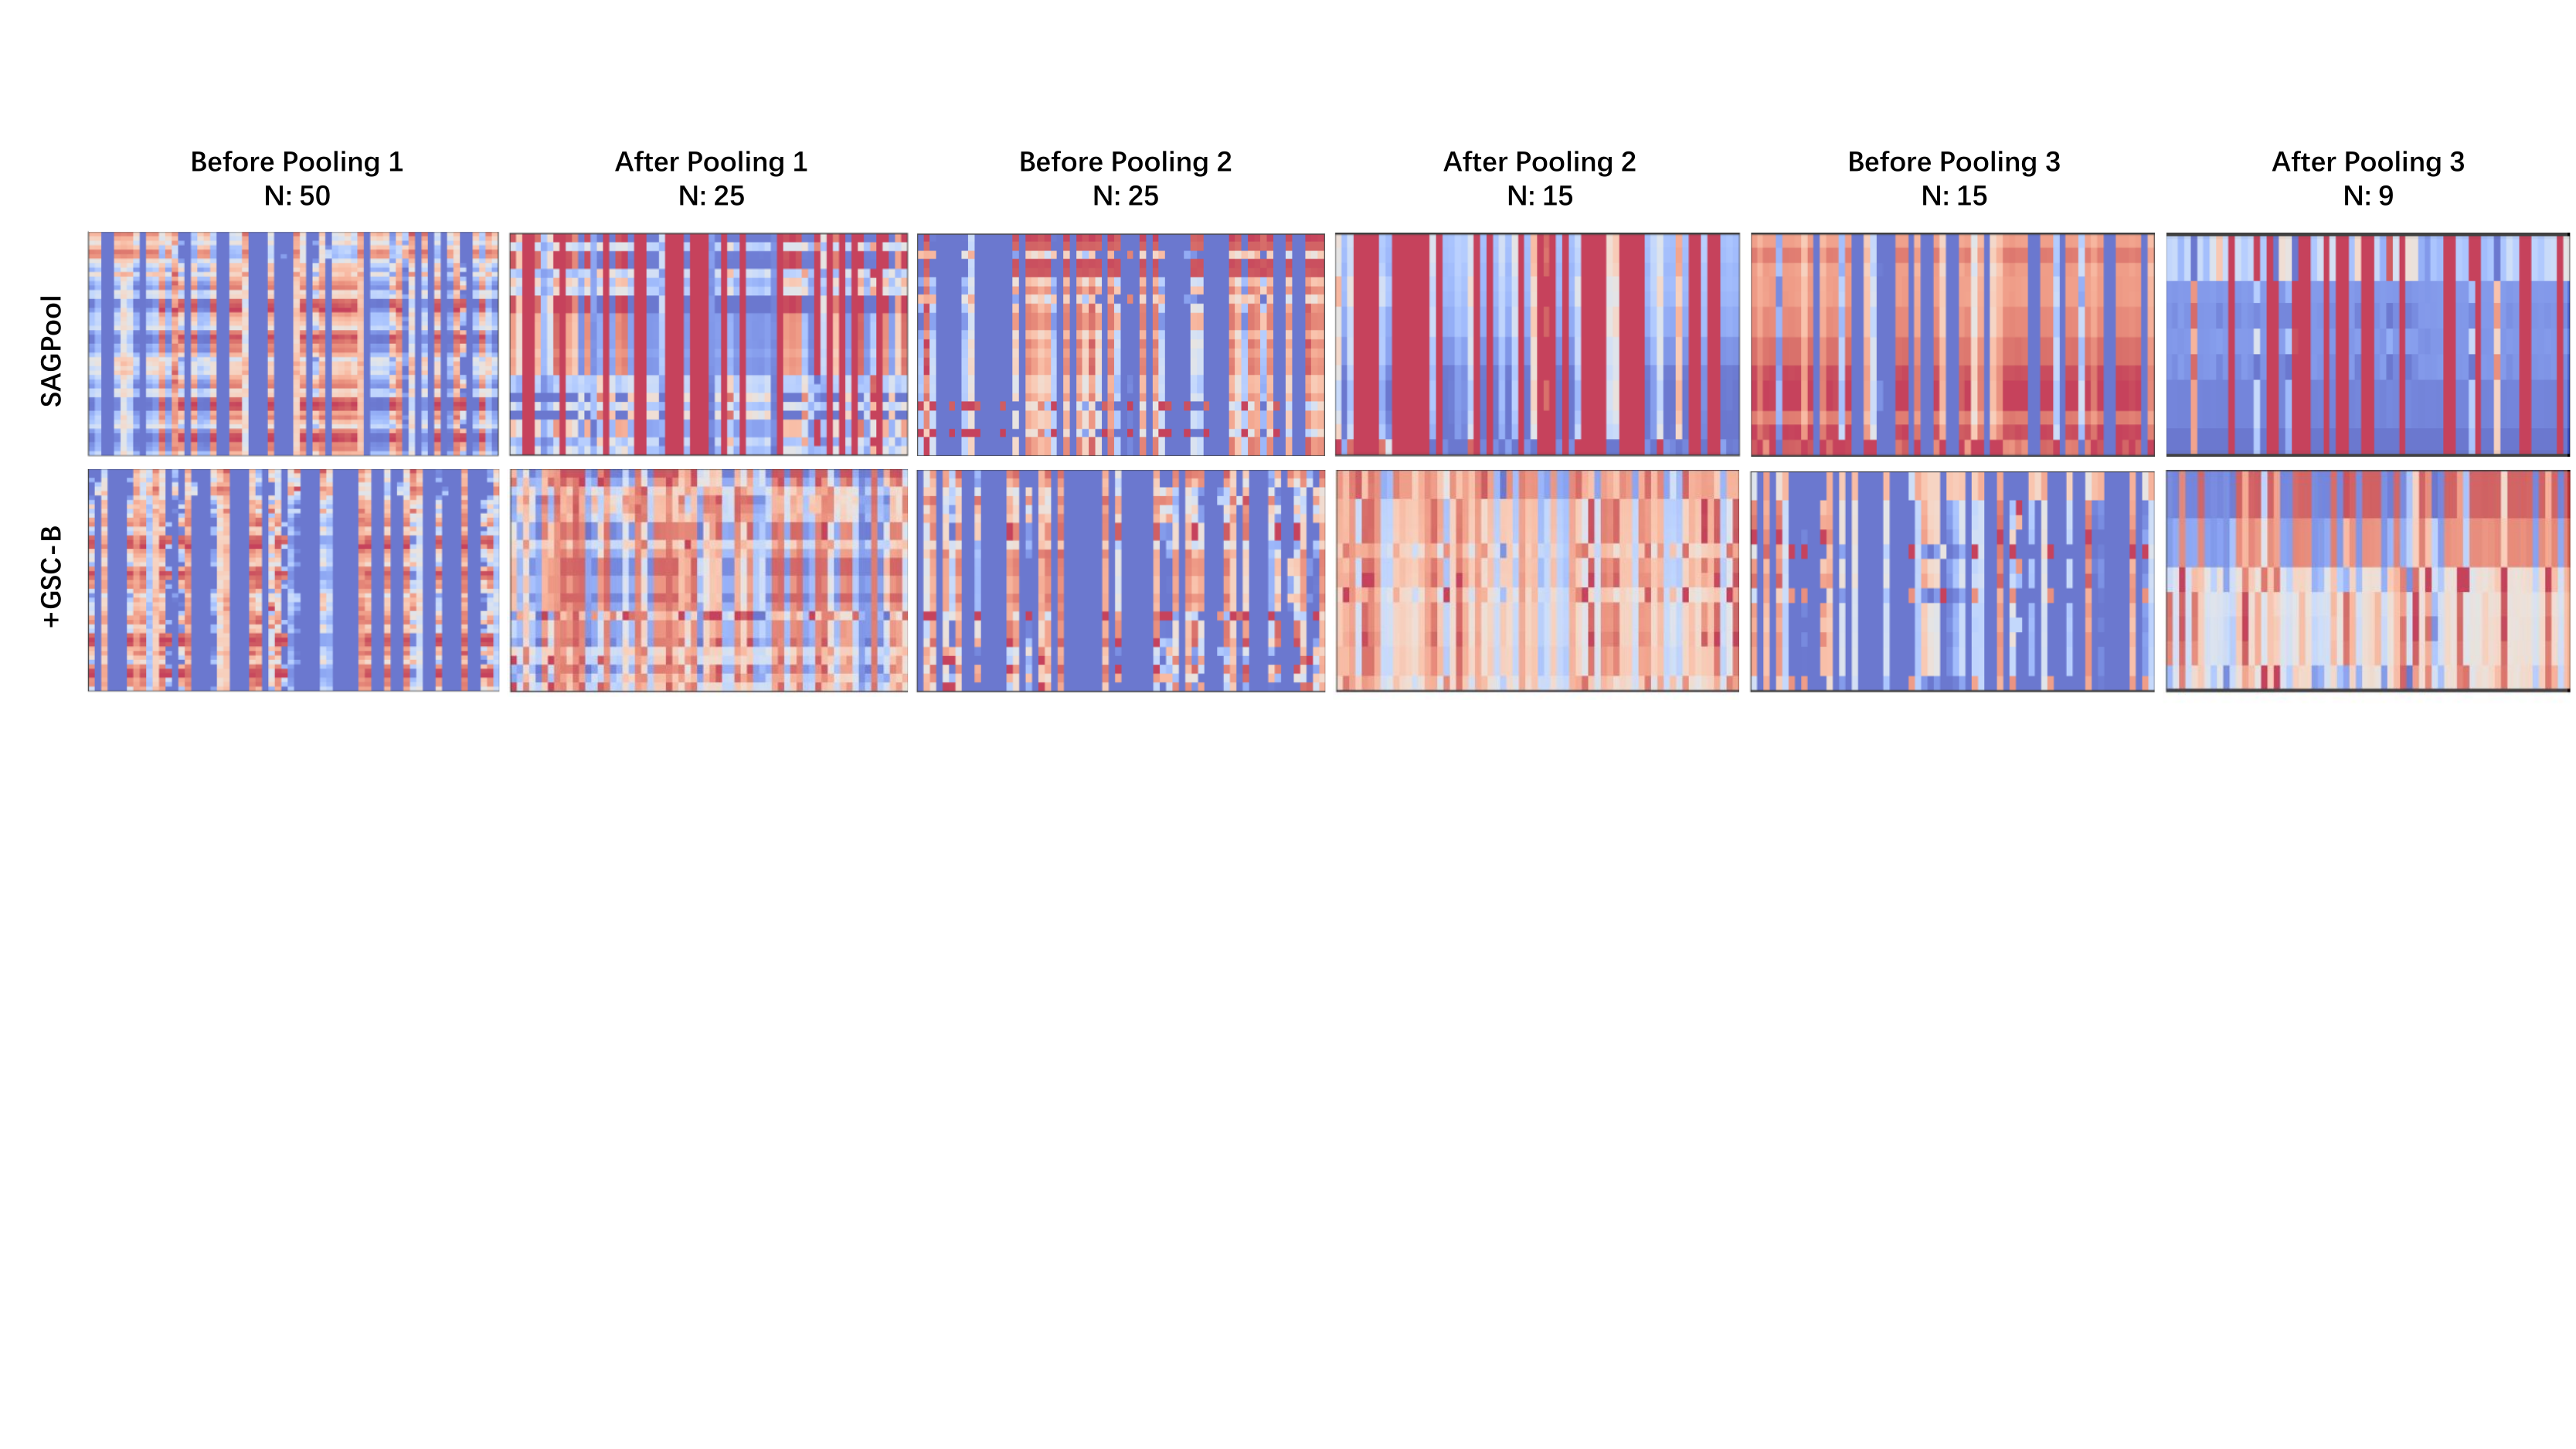}
%   \vspace{-2mm}
  \caption{Visualization of node embeddings  on SAGPool and GSC-B (SAGPool).
 }
 \label{fig:append-demo-1}
%  \vspace{-2mm}
\end{figure*}

\begin{figure*} [htbp]
  \centering
  % Requires \usepackage{graphicx}
  \includegraphics[width=0.7\linewidth]{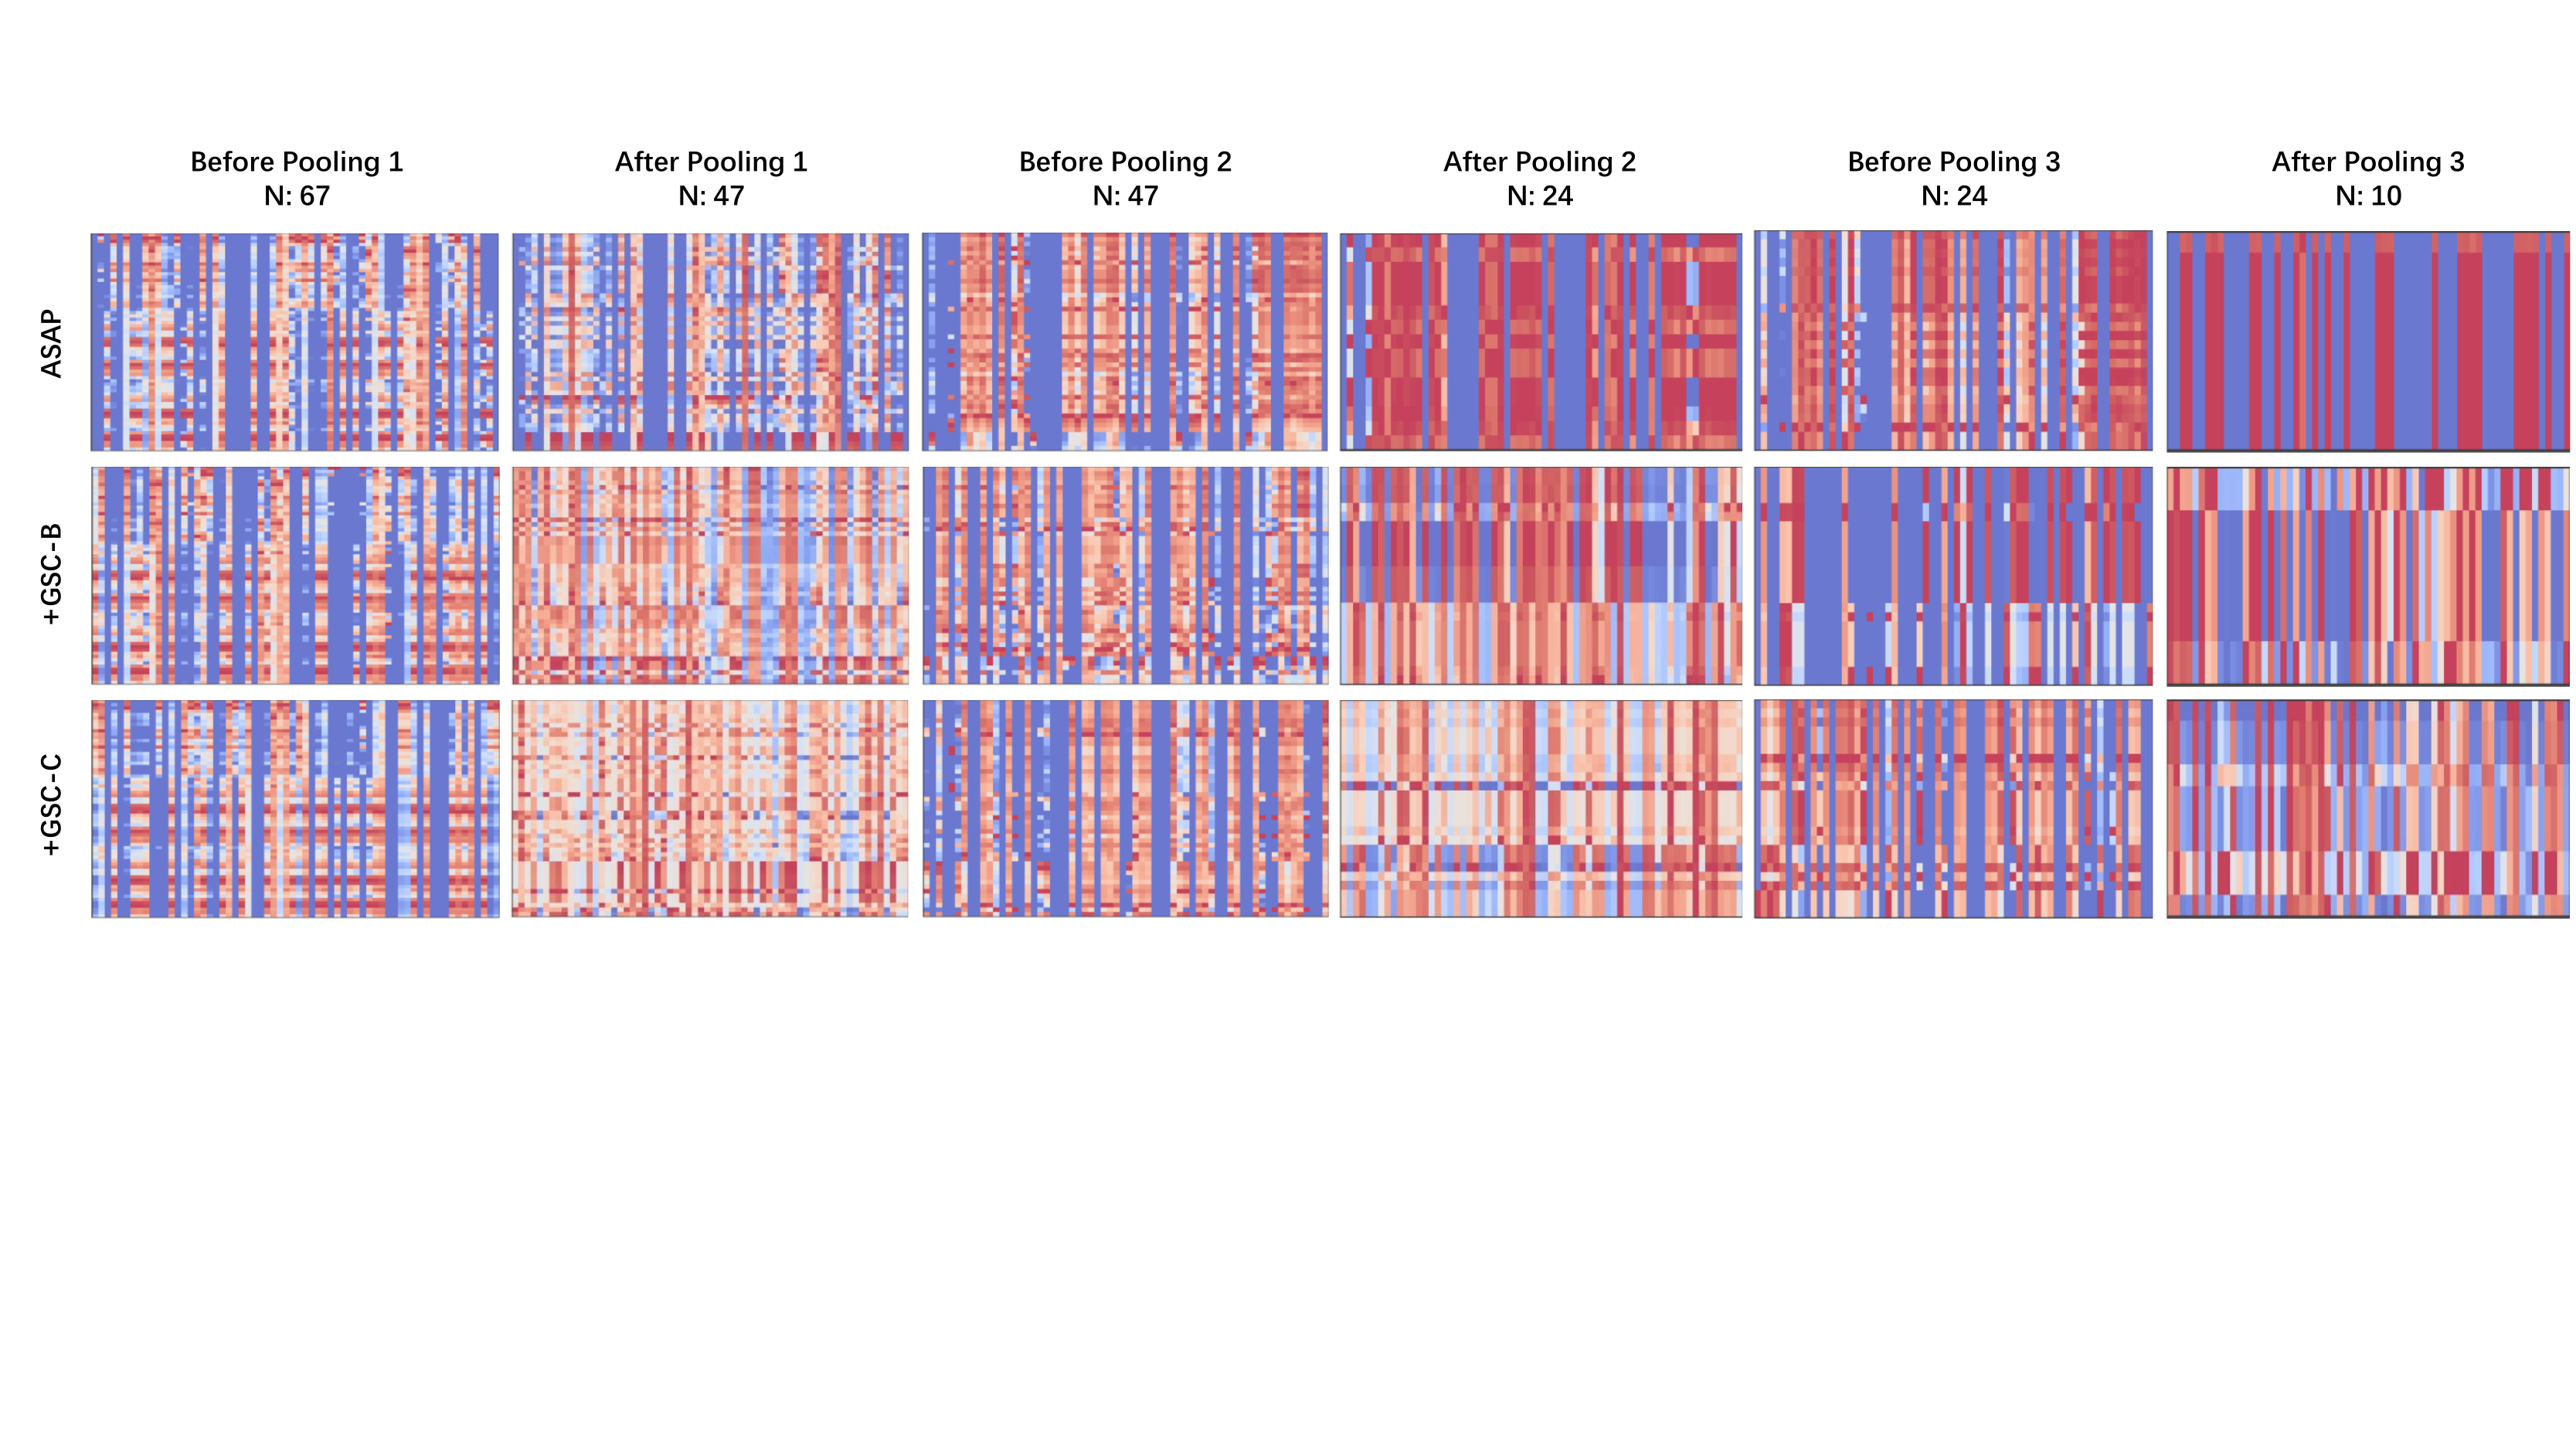}
%   \vspace{-2mm}
  \caption{Visualization of node embeddings on ASAP, GSC-B (ASAP) and GSC-C (ASAP).
 }
 \label{fig:append-demo-2}
%  \vspace{-2mm}
\end{figure*}
