# Supplementary material for: Diversified Multiscale Graph Learning with Graph Self-Correction
Source: arXiv:2103.09754 source file (2021-03-17)
Supplement: Supplementary file 2 [file appendix_framework.tex]

\begin{figure*} [h]
  \centering
  % Requires \usepackage{graphicx}
  \includegraphics[width=0.7\linewidth]{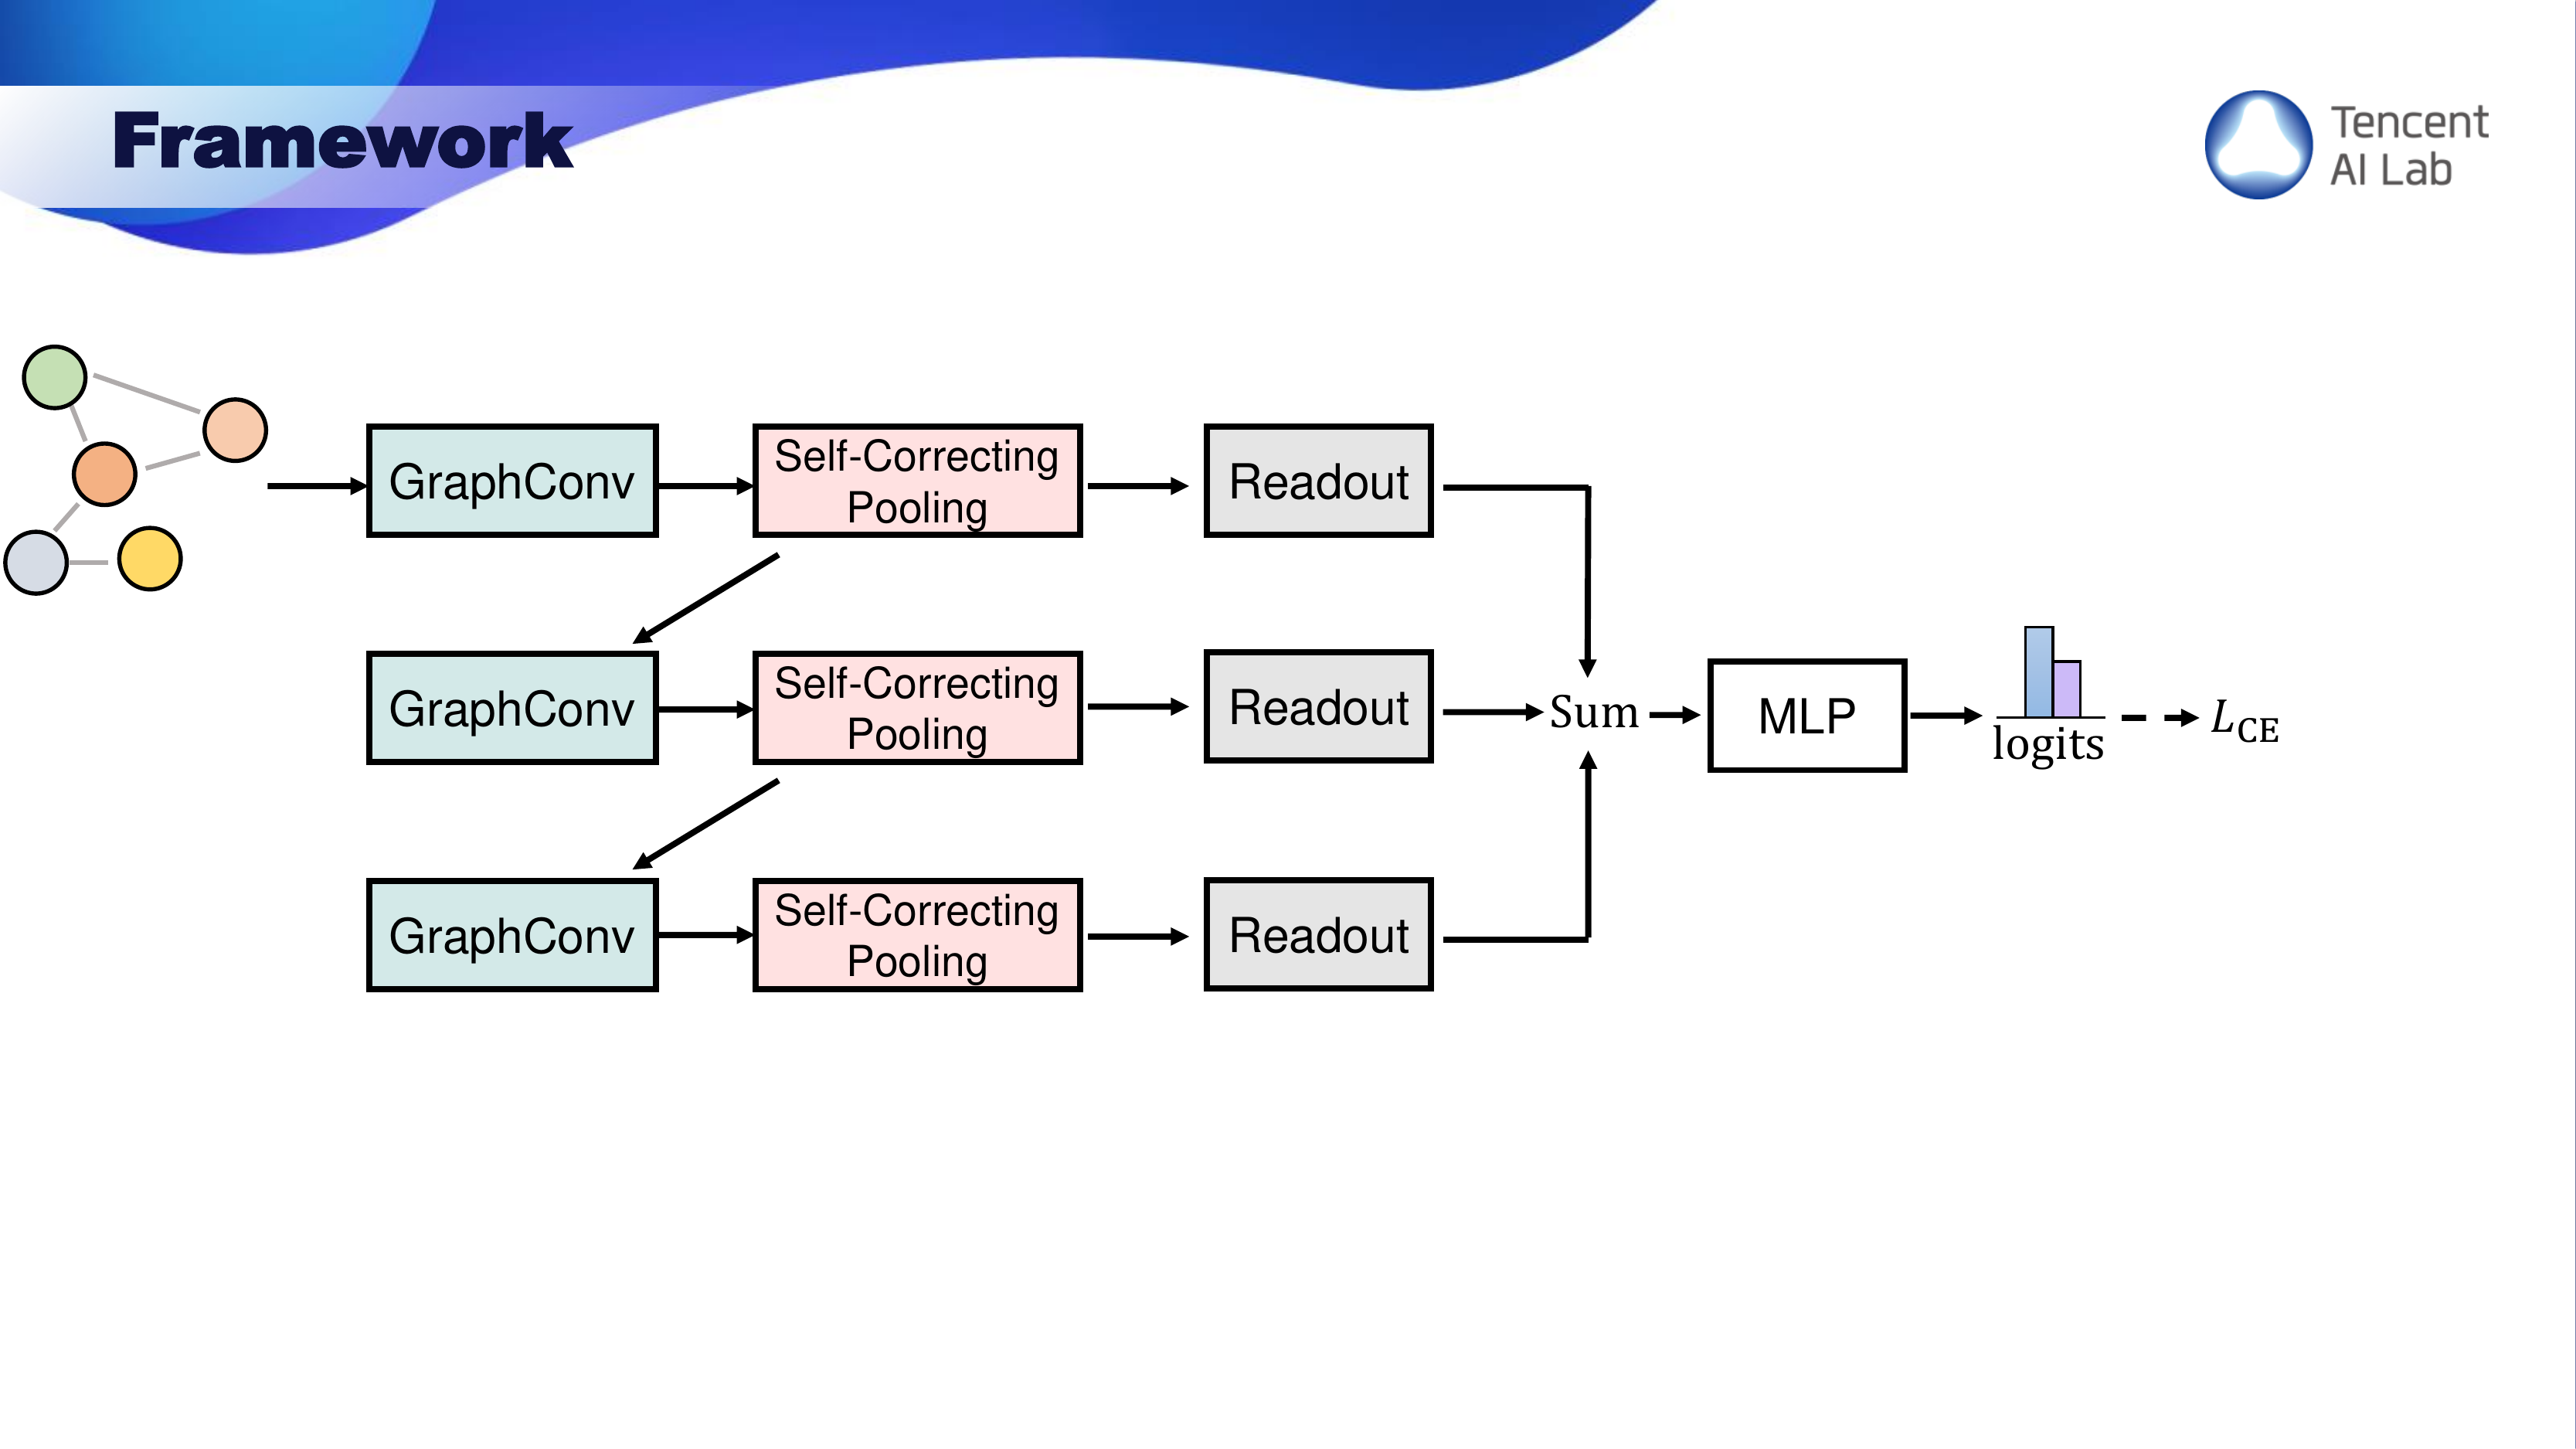}
%   \vspace{-2mm}
  \caption{The multiscale graph learning framework used for evaluating various pooling methods.
 }
 \label{fig:append_basebackbone} 
%  \vspace{-2mm}
\end{figure*}
