# Supplementary material for: Diversified Multiscale Graph Learning with Graph Self-Correction
Source: arXiv:2103.09754 source file (2021-03-17)
Supplement: Supplementary file 3 [file appendix_ogb.tex]

\begin{figure*} [h]
  \centering
  % Requires \usepackage{graphicx}
  \includegraphics[width=0.63\linewidth]{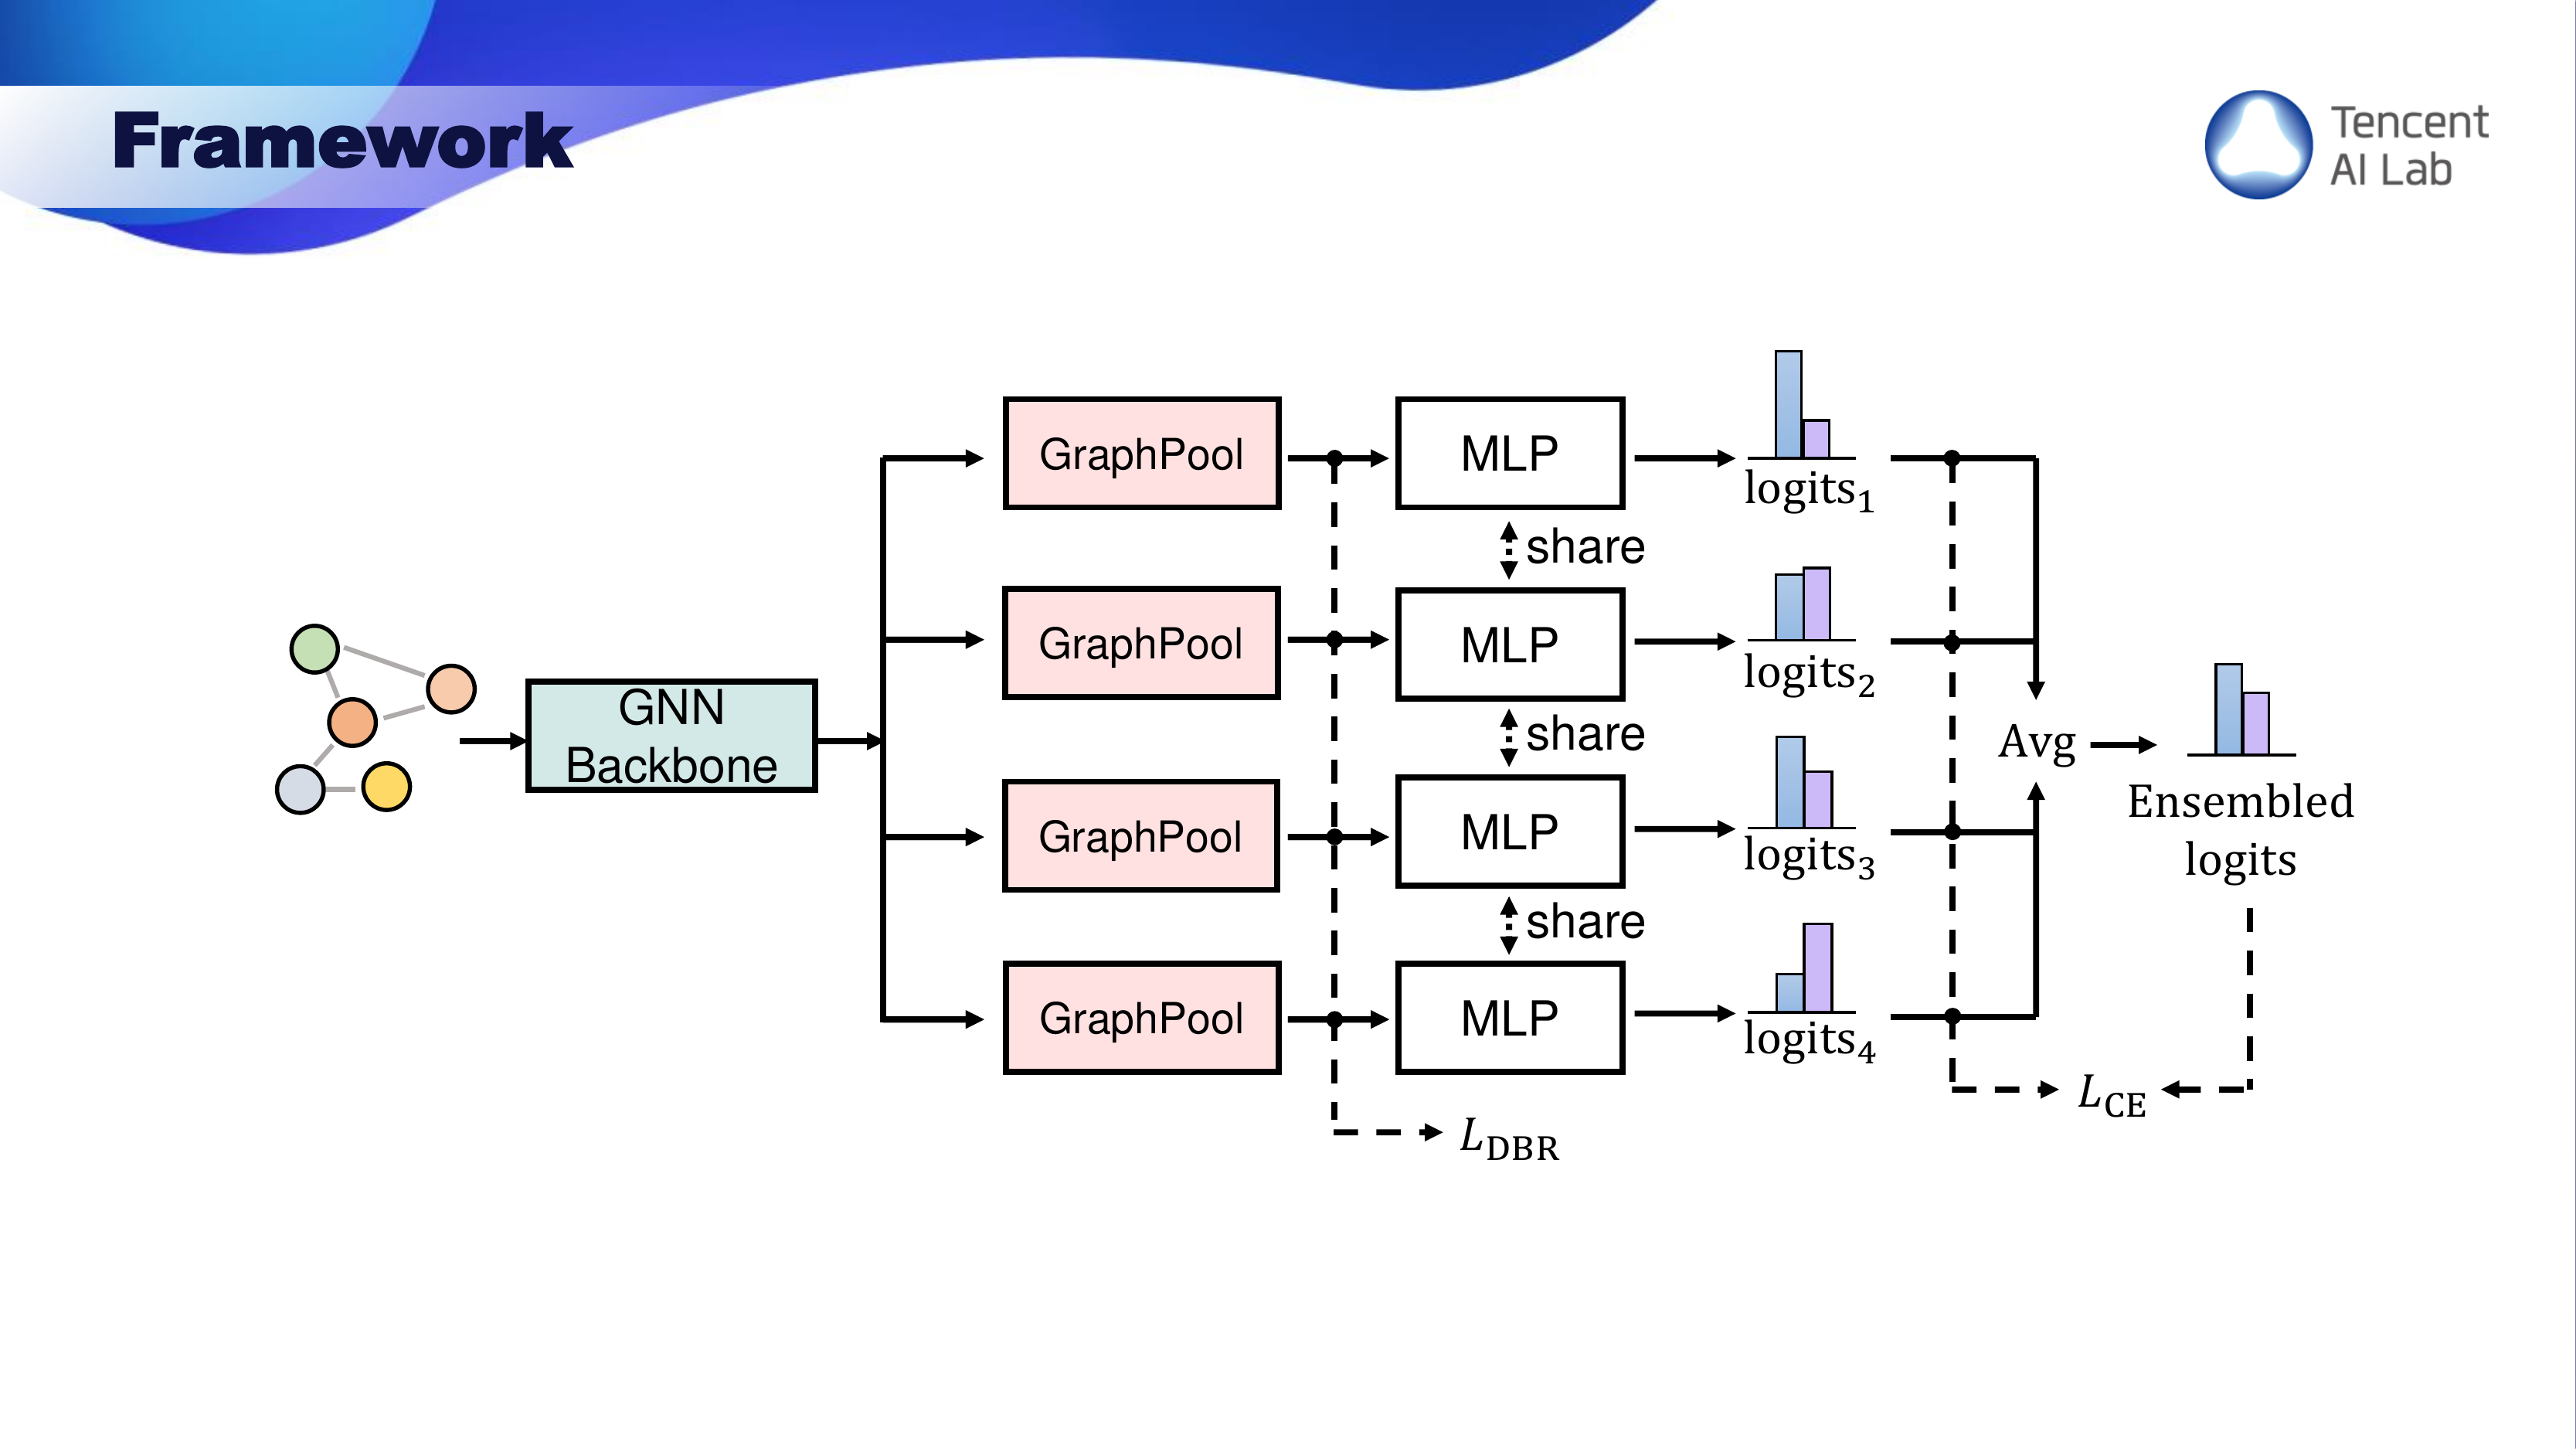}
%   \vspace{-2mm}
  \caption{The stacking-style ensemble model based on SOTA GNN backbones on MOLHIV.
 }
 \label{fig:append_ogb} 
%  \vspace{-2mm}
\end{figure*}
